# Supplementary material for: TraMNet - Transition Matrix Network for Efficient Action Tube Proposals
Source: arXiv:1808.00297 source file (2018-08-01)
Supplement: Supplementary file 1 [file supp_details.tex]

In this supplementary material, we first present implementation details in Section~\ref{subsec:details}.
Next, we show how optical flow and appearance based feature contribute to the final performance 
in Section~\ref{sec:Contribution}.
Finally, we show how the transition matrix helps in dynamic classes over AMTNet-L in Section~\ref{sec:classes}.

\section{Implementation details}\label{subsec:details}

All models are trained with a batch size of $16$ on two 1080Ti GPUs (11GB VRAM each) for AMTNet-L and TraMNet.
Whereas, ACT-L is trained on 4 GPUs because it requires fitting feature maps of 6 frame into GPU memory.
We used Pytorch library to implement all the models (ACT-L, AMTnet-L, and TraMNet) by following the implementation of Singh \etal \cite{singh2016online} closely from their
% \url{ GitHub repository}{https://github.com/gurkirt/realtime-action-detection}.
\href{https://github.com/gurkirt/realtime-action-detection}{GitHub repository}.

\textbf{UCF1101-24.} We trained all our models using the data-loader function provided by Singh \etal~\cite{singh2016online} where 5000 training images are picked for each class to train.
The RGB stream is trained with an initial learning rate of $0.001$ and it is dropped by a factor of $10$ after $110K$ iterations, and the model is trained for $180K$ iterations for all the different detection frameworks, i.e., ACT-L, AMTMet-L, and TraMNet.
The flow stream is trained with an initial learning rate of $0.001$ and it is dropped by a factor of $10$ after $150K$ iterations, and the model is trained for $220K$ iterations for all the different detection frameworks, i.e., ACT-L, AMTMet-L, and TraMNet.

\textbf{DALY.} We use all the action instances of actions available even if 
the number of frames annotated in a given instance is less than 2. AMTNet-L and 
TraMNet requires at least two consecutive frames to train, but in case of 
DALY dataset, there are action instances where only one frame is annotated, we use annotated 
frame twice to make a sequence of two frames, as mentioned in the paper 
this happens for $12\%$ of action instances.
Remaining instances contribute according to the number of frames annotated per instance.

The RGB stream is trained with an initial learning rate of $0.001$ and it is dropped by a factor of $10$ after $12K$ iterations, and the model is trained for $30K$ iterations for all the different detection frameworks, i.e., AMTNet-L and TraMNet.
The Flow stream is trained with an initial learning rate of $0.001$ and it is dropped by a factor of $10$ after $15K$ iterations, and the model is trained for $50K$ iterations for all the different detection frameworks, i.e., AMTNet-L and TraMNet.

\textbf{Input Data Preparations.}
The number of input video frames to CNNs is more than $1$ in our case, e.g., $6$ for ACT-L action detection framework. 
The optical flow stream uses a stack of 5 frames as input for each input training example in the sequence.
In our case, sequence length ($s$) is more than (in case AMTNet-L and TraMNet equal to 2 and ACT-L equal to 6), 
so 2 or 6 ($s=2$) stacks of 5 frames are used as input for flow stream in case of TraMNet for flow stream.

The number of input frames for the RGB stream is equal to the sequence length, e.g., 2 for TraMNet.
Each optical flow image is a 3 channel image, where first two channels are flow in  $x$ and $y$ direction respectively and the third channel is the magnitude (square-root of the sum of squares) of flow in both directions.
We computed dense optical flow between each pair of successive video frames using the algorithms of~\cite{Brox-2004}.

The SSD relies on \textbf{data augmentation} to boost the performance, we extended the data augmentation~\cite{liu15ssd} function provided by Singh \etal \cite{singh2016online} in  their
\href{https://github.com/gurkirt/realtime-action-detection}{GitHub repository} to pass as input a sequence of frames in place of a single frame.
The same data augmentation was applied to all the frames in a training batch.

\textbf{VGG weight initialisation.}
The weights of VGG network (base network) are initialised with weights from a pre-trained ImageNet model~\cite{liu2015parsenet}\footnote{\url{https://gist.github.com/weiliu89/2ed6e13bfd5b57cf81d6}}
for appearance- and flow-based SSD networks for both UCF101-24 and DALY dataset.

\section{RGB and Flow Contribution}\label{sec:Contribution}
In Figure~\ref{table:ucf101_contrib}, we show how each stream individually performs and contributes the performance of fused model using \textit{mean-fusion}~\cite{kalogeiton2017action}.
We can observe that the RGB stream works better than the flow stream and fusion always gives improvements over the RGB stream.
Interestingly, the RGB stream is most dominant and performs comparable to the fusion model, hence one can only use RGB stream to improve the run-time speed of the whole system at the cost of a small performance drop.

\begin{table}[t]
  %\vskip -3mm
  \centering
  \setlength{\tabcolsep}{3.5pt}
  \caption{Action localisation results on untrimmed videos from UCF101-24 split1.
  The table is divided into 4 parts. The first part lists approaches which have single frames as input;
  the second part approaches which take multiple frames as input;
  the third part contemplates the reimplemented versions of approaches in the second group;
  lastly, we report TraMNet's performance.}
  \vskip 1mm
  {\footnotesize
  \scalebox{1}{
  \begin{tabular}{lccccccc}
  \toprule
  Methods & Train $\Delta$ & Test $\Delta$	&$\delta$ = 0.2   &$\delta$ = 0.5 & $\delta$ = 0.75 & $\delta$ = .5:.95 & Acc \% \\ \midrule
  %Yu \etal~\cite{yu2015fast} &NA &NA & 26.5  & --   & -- & -- & --\\
  %Weinzaepfel ~\cite{Weinzaepfel-2015}  & NA &NA & 46.8  & --   & -- & -- & --\\
  T-CNN~\cite{hou2017tube} & NA &NA & 47.1  & --   & -- & -- & --\\
  MR-TS~\cite{peng2016eccv}	 & NA &NA & 73.5  & 32.1 & 02.7 & 07.3 & --\\
  Saha~\etal~\cite{Saha2016}    & NA &NA & 66.6  & 36.4 & 07.9 & 14.4 & --\\
  SSD~\cite{singh2016online}    & NA & NA & 73.2 & 46.3 & 15.0 & 20.4 & --\\\midrule
  AMTnet~\cite{saha2017amtnet} rgb-only  & 1,2,3 & 1 & 63.0  & 33.1 & 00.5 & 10.7 & --\\
  ACT~\cite{kalogeiton2017action}   & 1 & 1 & 76.2  & 49.2 & 19.7 & 23.4 & --\\
  Gu \etal~\cite{ava2017gu} (\cite{peng2016eccv} + \cite{carreira2017quo})   & NA & NA & --  & \textbf{59.9} & -- & -- & --\\
  \midrule
  SSD-L with-trimming  & NA & NA & 76.2 & 45.5 & 16.4 & 20.6  & 92.0 \\
  SSD-L     & NA & NA & 76.8 & 48.2 & 17.0 & 21.7  & 92.1 \\
  ACT-L RGB               & 1 & 1 & 74.2 & 47.9 & 18.6 & 22.4  & 88.0 \\
  ACT-L Flow              & 1 & 1 & 72.8 & 43.9 & 12.3 & 18.6  & 86.2 \\
  ACT-L RGB+Flow          & 1 & 1 & 77.9 & 50.8 & 19.8 & \textbf{23.9}  & 91.4 \\
  AMTnet-L RGB            & 1 & 1 & 76.2 & 46.9 & 18.0 & 21.9  & 89.1 \\
  AMTnet-L Flow           & 1 & 1 & 73.7 & 43.6 & 11.3 & 17.5  & 88.2 \\
  AMTnet-L RGB+Flow       & 1 & 1 & \textbf{79.4} & \textbf{51.2} & 19.0 & 23.4  & \textbf{92.9} \\ \midrule
  TraMNet (ours) RGB      & 1 & 1 & 76.8 & 46.9 & 18.9 & 22.2  & 88.5 \\
  TraMNet (ours) Flow     & 1 & 1 & 74.9 & 43.1 & 11.2 & 17.6  & 87.1 \\
  TraMNet (ours) RGB+FLow & 1 & 1 & 79.0 & 50.9 & \textbf{20.1} & \textbf{23.9}  & 92.4 \\\bottomrule
  \end{tabular}
  }
  }
  %\vspace*{-\baselineskip}
  \label{table:ucf101_contrib} \vspace{-5mm}
\end{table}

\section{Ablation Study: Performance on Classes with Movements}\label{sec:classes}
There are many action classes with a lot of spatial movement in the UCF101-24 dataset, unlike DALY dataset where only ``CleaningFloor'' had spatial movements.
In Table \ref{table:ablation-study-ucf10102}, we show class-wise performance at detection threshold $\delta=0.2$.
We consider a class to have a considerable spatial movements if the class contributes to the off-diagonal elements in the transition matrix at $\Delta = 5$.
The ``BasketballDunk'', ``Skiing'', ``VolleyballSpiking'' are the classes which contribute most to the off-diagonal entries in the transition matrix.
It is clear from the Table \ref{table:ablation-study-ucf10102} that the transition matrix helps to improve the detection performance considerably for those classes (highlighted in red) which have signifiacnt spatial movements.
It is important to note that we build a transition matrix for each scale separately, our method is limited in case of when an actor moves towards or away from camera, or camera moves in that direction.
One such case is biking observed from the front view of the biker.
Solution to cover such movements is to build one transition matrix for all the pyramids.
However, our base network is SSD, which has inconsistent feature dimension across the scales of the pyramid, hence, concatenated features from different scales would result in inconsistent dimensionality.

The classes with multiple actors (e.g. ``IceDancing'', ``SalsaSpin'', ``Fencing'') suffer in the TraMNet framework.
We think it is due to the fact that the anchor micro-tubes are 
class invariant and movement of some classes might be creating confusion in these classes.
Adding class-specific anchor micro-tubes and respectively 
making regression layers class specific could help alleviate this problem.
In some static classes (e.g. ``GlofSwing'' or ``TennisSwing'')
we observe that TraMNet is better than both ACT-L and AMTNet-L, 
where as in other static classes (e.g. ``CricketBowling'' and ``RopeClimbing''), ACT-L is better.
We think it because ACT uses features from 6 frames and able to classify the classes better.

\begin{table*}
\vspace{5mm}
\centering
\footnotesize
\caption{Spatio-temporal detection results (video APs in $\%$) on UCF101-24 at $\delta=0.2$. Classes with movement in the dataset are highlighted in red colour.  }
\scalebox{0.60}{
\begin{tabular}{lcccccccc}
\toprule
%%%%%%%%%%%%%%%%%%%%%%%%%%%%%%%%%%%%%%%%%%%%%%%%%%%%%%%%%%%%%%%%%%%%%%%%%%%
%%%%%%%%%%%%%%%%%%%%%%%%%%%%%%%%%%%%%%%%%%%%%%%%%%%%%%%%%%%%%%%%%%%%%%%%%%%
Actions		     		& Basketball  &   \red{BasketballDunk} &   Biking &   \red{CliffDiving} &   CricketBowling &   \red{Diving} &   Fencing & \red{FloorGymnastics}  \\ \midrule
ACT-L & 50.3 & 78.0 & 78.3 & 79.2 & 70.5 & 100.0 & 89.9 & 98.9 \\
AMTNet-L & 53.6 & 79.4 & 82.2 & 81.7 & 65.7 & 100.0 & 90.7 & 99.5 \\
TraMNet & 51.9 & 81.8 & 80.0 & 81.6 & 60.6 & 100.0 & 87.0 & 98.8 \\ \midrule \midrule
Actions 			& GolfSwing   &   HorseRiding & IceDancing &   \red{LongJump} & PoleVault &   RopeClimbing &   SalsaSpin &  SkateBoarding \\ \midrule
%%%%%%%%%%%%%%%%%%%%%%%%%%%%%%%%%%%%%%%%%%%%%%%%%%%%%%%%%%%%%%%%%%%%%%%%%%%
%%%%%%%%%%%%%%%%%%%%%%%%%%%%%%%%%%%%%%%%%%%%%%%%%%%%%%%%%%%%%%%%%%%%%%%%%%%
ACT-L & 69.8 & 96.1 & 87.9 & 81.9 & 88.9 & 99.4 & 43.6 & 89.8 \\
AMTNet-L & 77.6 & 96.1 & 86.5 & 88.6 & 92.9 & 98.1 & 46.9 & 88.0 \\
TraMNet & 76.5 & 96.1 & 83.5 & 86.6 & 88.8 & 97.7 & 41.7 & 89.2 \\  \midrule \\ \midrule
Actions  &   \red{Skiing} & \red{Skijet} & SoccerJuggling & Surfing & TennisSwing & TrampolineJumping & \red{VolleyballSpiking} & WalkingWithDog  \\ \midrule
%%%%%%%%%%%%%%%%%%%%%%%%%%%%%%%%%%%%%%%%%%%%%%%%%%%%%%%%%%%%%%%%%%%%%%%%%%%
%%%%%%%%%%%%%%%%%%%%%%%%%%%%%%%%%%%%%%%%%%%%%%%%%%%%%%%%%%%%%%%%%%%%%%%%%%%
ACT-L & 81.1 & 87.8 & 95.0 & 67.0 & 35.0 & 67.6 & 44.0 & 90.4 \\
AMTNet-L & 82.4 & 93.5 & 94.9 & 68.9 & 40.5 & 65.7 & 42.0 & 90.4 \\
TraMNet & 85.2 & 93.6 & 94.4 & 65.6 & 42.8 & 66.8 & 53.5 & 91.2 \\
%%%%%%%%%%%%%%%%%%%%%%%%%%%%%%%%%%%%%%%%%%%%%%%%%%%%%%%%%%%%%%%%%%%%%%%%%%%
\bottomrule
\end{tabular}
}
\label{table:ablation-study-ucf10102}
\end{table*}
